# Supplementary material for: A statistical model for brain networks inferred from large-scale electrophysiological signals
Source: arXiv:1611.06893 ancillary file (2017-02-17)
Supplement: Supplementary file 1 [file Supp_Text.pdf]

**Supplementary Text**

Our main results pointed out the role of the segregation of information (i.e., local-efficiency) in the *alpha* band. This specific band is known to be the most prominent in resting state conditions [1]. However, it is possible that the selected threshold belongs to a larger interval for which differences can still be appreciated. Figure 1 (right panel), shows that local-efficiency was significantly different between conditions ($p < 0.001$) only for $k = 3$ and $k = 5$, while global-efficiency (left panel) never reached significance for any other $k$ value corresponding to the typically explored ranges of density thresholds [2] (i.e., max density=0.4 or equivalently k=22 in our study).

We then evaluated our modeling approach for $k = 5$. The ranking of the ERGM models followed the same tendency that as for $k = 3$. $M_1$ gave the lowest $\delta(E_g, E_l)$ scores as compared to other configurations (Figure 2). As for $k = 3$, model $M_1$ for $k = 5$ gave a good model adequacy (Figure 3) and cross-validation over different graph indices (Figure 4 and 5)

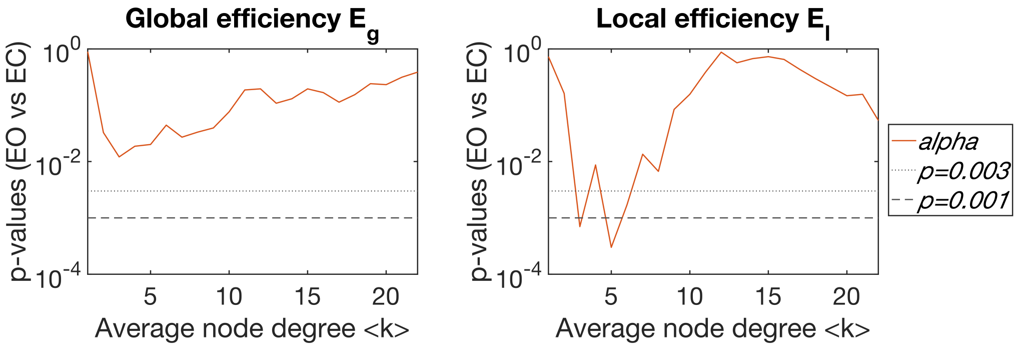


Figure 1: Statistical differences for global- and local-efficiency across different threshold values. $p$-values result from permutation t-tests between EO and EC conditions in the *alpha* frequency band. Thresholds are shown as a function of the average node degree $k$.

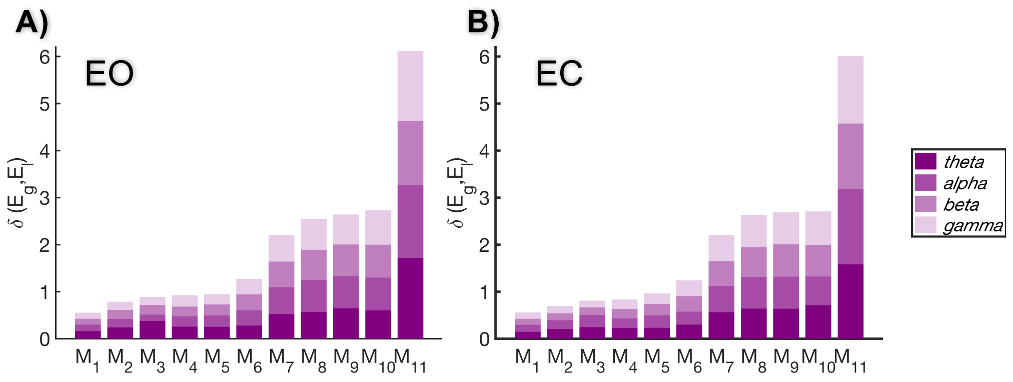


Figure 2: Absolute quality of ERG models' fit for networks thresholded with $k = 5$. Colored bars show the group-averaged cumulative errors $\delta(E_g, E_l)$ in terms of relative of global- and local-efficiency across frequency bands. Model configurations are listed on the x-axis. Panel A) illustrates values for eyes-open resting-state (EO); panel B) shows the error values for eyes-closed resting-state (EC).

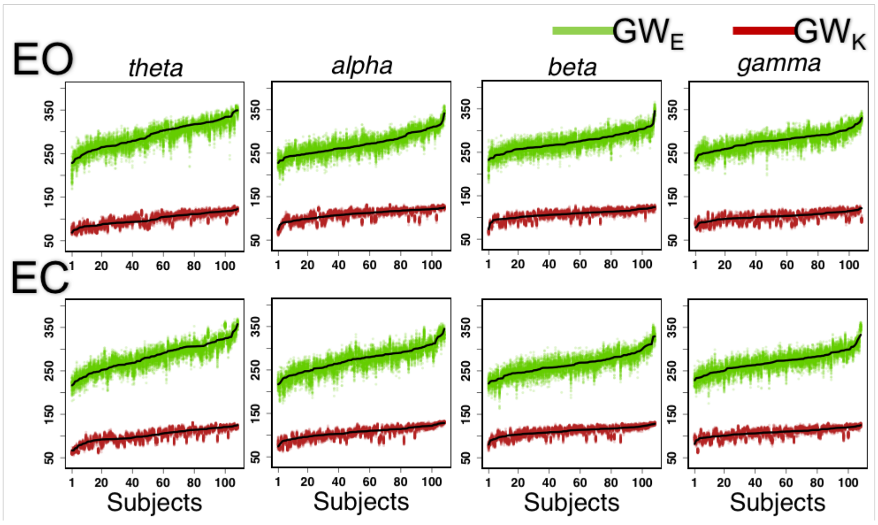


Figure 3: Adequacy of model configuration $M_1$ for networks thresholded with $k = 5$. Green and red dots represent respectively the values of the *geometrically weighted edgewise shared pattern distribution* ($GW_E$) and *geometrically weighted degree distribution* ($GW_K$) measured in simulated networks. Black dots lines indicate the values measured in the observed brain networks.

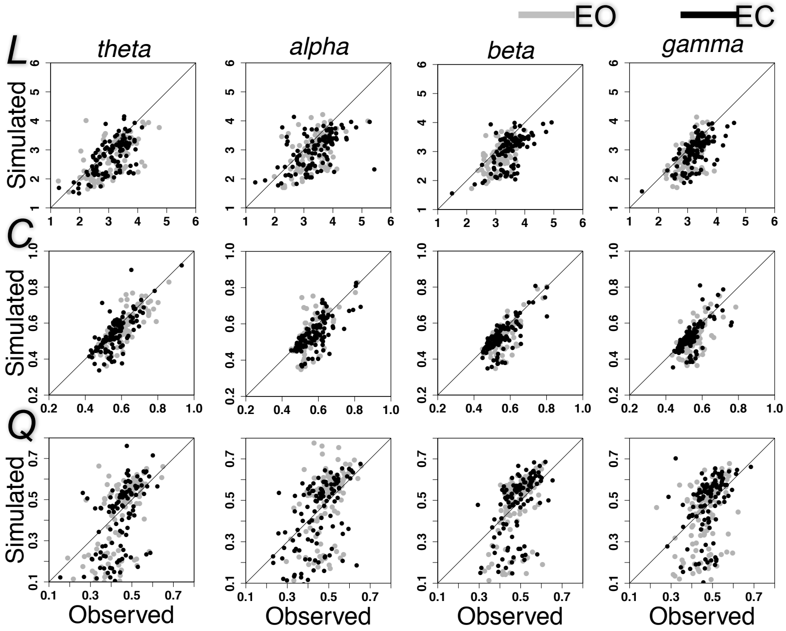


Figure 4: Cross-validation for model configuration $M_1$ for networks thresholded with $k = 5$. Scatter plots show the values of the graph indices measured in the observed brain networks (x-axis) against the mean values obtained from synthetic networks (y-axis). Three graph indices were considered: characteristic path length ($L$), clustering coefficient ($C$) and modularity ($Q$). Grey dots correspond to eyes-open resting-states (EO); black dots correspond to eyes-closed resting-states (EC).

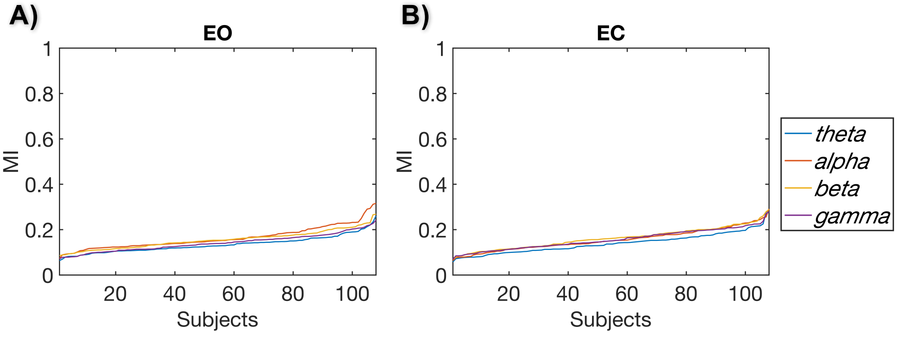


Figure 5: Mirkin index (MI) between partitions of observed networks and a consensus partition of the synthetic networks for $k = 5$. We selected $\tau = 1$ as a resolution parameter to construct the consensus partition. Similar results were obtained for $\tau > 1$ (data not shown here)

[1] W. Klimesch, Alpha-band oscillations, attention, and controlled access to stored information, Trends in Cognitive Sciences 16 (12) (2012) 606–617. doi:10.1016/j.tics.2012.10.007.
URL http://www.ncbi.nlm.nih.gov/pmc/articles/PMC3507158/

[2] K. A. Garrison, D. Scheinost, E. S. Finn, X. Shen, R. T. Constable, The (in)stability of functional brain network measures across thresholds, NeuroImage 118 (2015) 651–661. doi:10.1016/j.neuroimage.2015.05.046.
